# Supplementary material for: GeCoNeRF: Few-shot Neural Radiance Fields via Geometric Consistency
Source: arXiv:2301.10941 source file (2023-04-27)
Supplement: Supplementary file 1 [file supple.tex]

Here we provide more implementation details (Section~\ref{details}) and a pseudo-code describing algorithm of consistency modeling in GeCoNeRF (Section~\ref{algo}). Next, in Section~\ref{cons}, we give an additional ablation study of our method, to differentiate our work to existing methods that utilize multiview consistency. In Section~\ref{viewnum}, we give an experimental quantitative analysis of our model regarding the number of input images given to the model, in comparison with our baseline model. Finally, in Section~\ref{limitations}, we give our analysis of our model's performance and the limitations of our method. 

\section{More Implementation Details}
\label{details}
\paragraph{Network architecture.}
We use mip-NeRF~\cite{mildenhall2020nerf} as network backbone and our neural radiance field is paramterized as fully connected ReLU network with hidden dimension of 256 and depth of 8 layers. We use 128 samples along the ray for both coarse and fine sample levels. Our model is implemented using the PyTorch framework~\cite{lin2020nerfpytorch} on top of the pytorch-NeRF code base~\cite{lin2020nerfpytorch}. \vspace{-5pt}

\paragraph{Training details.}  
We train our neural networks using ADAM optimizer~\cite{kingma2015adam}. The learning rate is first linearly warmed up from 0 to $5\times 10^{-4}$ for the first 5k iterations, and then controlled by the cosine decay schedule to the minimum learning rate of $5\times 10^{-6}$. We clip gradients by value at 0.1 and then by norm at 0.1. We train each model for 70k iterations for 6 hours in total on a two Nvidia 3090Ti GPU. We write the optimization algorithm for GeCo-NeRF's unobserved viewpoint consistency modeling as follows in Algorithm 1.   \vspace{-5pt}

\paragraph{Unseen view patch generation.}
The pose for novel viewpoints are generated by adding a small divergence angle to the pose of a randomly selected given input pose. For each iteration, divergence angle is uniformly sampled within a range value that linearly increases as a function of iteration steps. We convert the ground truth 4-by-4 pose matrix into Euler angles, and add the sampled divergent angle values to x- and y-axis Euler angle vector components. The z-axis component of Euler angle vector remains zero to prevent roll rotation from occurring. Then we convert the divergent angle back into pose matrix and generate corresponding rays with the same module used to generate ground truth viewpoint rays. We generate $120 \times 120$ sized patchwise rays by bilinearly upsampling $60 \times 60$ rays in a strided grid.

\paragraph{Novel pose sampling scheme.}
Our training details regarding pose sampling are as follows: we generate unobserved viewpoints by sampling camera location and poses on a half-sphere, with camera direction always directed towards its center, just like ground truth camera orientations given in our datasets. For progressive camera pose sampling, we sample noise value uniformly within interval of {[-d, +d]} and add it to the original Euler rotation angles of reference poses. Sampling range parameter d grows linearly from 3 to 9 degrees throughout the course of optimization. This has an effect of generating viewpoints progressively further away from original reference viewpoints as training steps increase.

\paragraph{Consistency loss weight decay.}
Due to divergent behaviours that are shown by NeRF as it undergoes few-shot optimization, and to match different rates of decrease between vanilla NeRF loss and consistency modeling loss, we add a weighting hyperparameter to our regularization loss. We find that this scheme is effective in preventing the regularization loss from growing out of proportion and degrading the reconstruction quality. We exponentially decay the loss weight with decay parameter as 20000, which indicates that decay weight result 0.367 when the number of iteration steps reach the said number.  

\newpage

\section{Algorithm}
\label{algo}

We present the algorithm of consistency modeling in GeCoNeRF as follows in Algorithm 1. Considering a depth image rendered by the NeRF model, $D_{j}$ at unseen viewpoint $j$. By formulating a warping function $\psi(I_{i};D_{j},R_{i \rightarrow j})$ that warps an image $I_{i}$ according to the depth $D_{j}$ and viewpoint difference $R_{i \rightarrow j}$, we can encourage a consistency between warped image $I_{i \rightarrow j} = \psi(I_{i};D_{j},R_{i \rightarrow j})$ and rendered image $I_{j}$ at $j$-th unseen viewpoint, which in turn improves the few-shot novel view synthesis performance.

%\vspace{-8}
% \usepackage[ruled,vlined]{algorithm2e}

\begin{algorithm}[H]
\SetAlgoLined

\textbf{initialization;}\;  {

 \While{$i$ $<$ $N$}{
  \For{$j\gets1$ \KwTo $m-1$}{
    $\alpha \gets \exp\left(-\sigma_\theta\left(g_i(\bm{p}(\hat{z}_j))\right)\cdot \Delta_j\right) \\
    \bm{c} \gets \bm{c}_\theta\left(g_i(\bm{p}(\hat{z}_j)) \bm{v}\right)$\ \\
    $\bm{C}_{u} \gets \bm{C}_{u} + A\cdot(1-\alpha)\cdot \bm{c} \ \ \ \\
    D_{j} \gets D_{j} + A\cdot(1-\alpha)\cdot\hat{d}_j \ \ \ \\
    A \gets A \cdot \alpha
    $\ }
  
  \If{regularization step}{
   \textbf{Backprojection:} $x \gets {D}_j(p_j)K^{-1}p_j$ \\
    \textbf{Reprojection:} $p_{j \rightarrow i} \gets KR_{j\rightarrow i}x$ \\
    \textbf{Inverse warping:} \\ $I_{i \rightarrow j}(p_i) \gets \mathrm{sampler}(I_{i};p_{j \rightarrow i})$ \\
    \textbf{Mask generation:} \\ $ M(p_j) \gets \big[\Vert {D}_j(p_j) - {D}_i(p_{j \rightarrow i}) \Vert < \tau\big]$ \\
    \textbf{Regularization loss calculation:} \\ $\mathcal{L}^{M}_\mathrm{cons} \gets \sum^L_{l=1} {1 \over C_l m_l}  \norm{ M_l \odot (f_\phi^l(I_{i \rightarrow j}) - f_\phi^l(I_j))}$   
   }{
  }
    Minimize $\mathcal{L}^{M}_\mathrm{cons}$\;}

 }
 \caption{GeCoNeRF Framework}
\end{algorithm}

\section{Comparison to Consistency Modeling Between Known Views}
%\vspace{-5pt}
\label{cons}

% : namely, \textbf{feature-level} consistency modeling at \textbf{novel viewpoints} with warped image as \textbf{pseudo GT}, along with \textbf{pixel-level occlusion handling}. 
\begin{wrapfigure}{r}{0.35\textwidth}\vspace{-19pt}
  \begin{center}
    \includegraphics[width=0.34\textwidth]{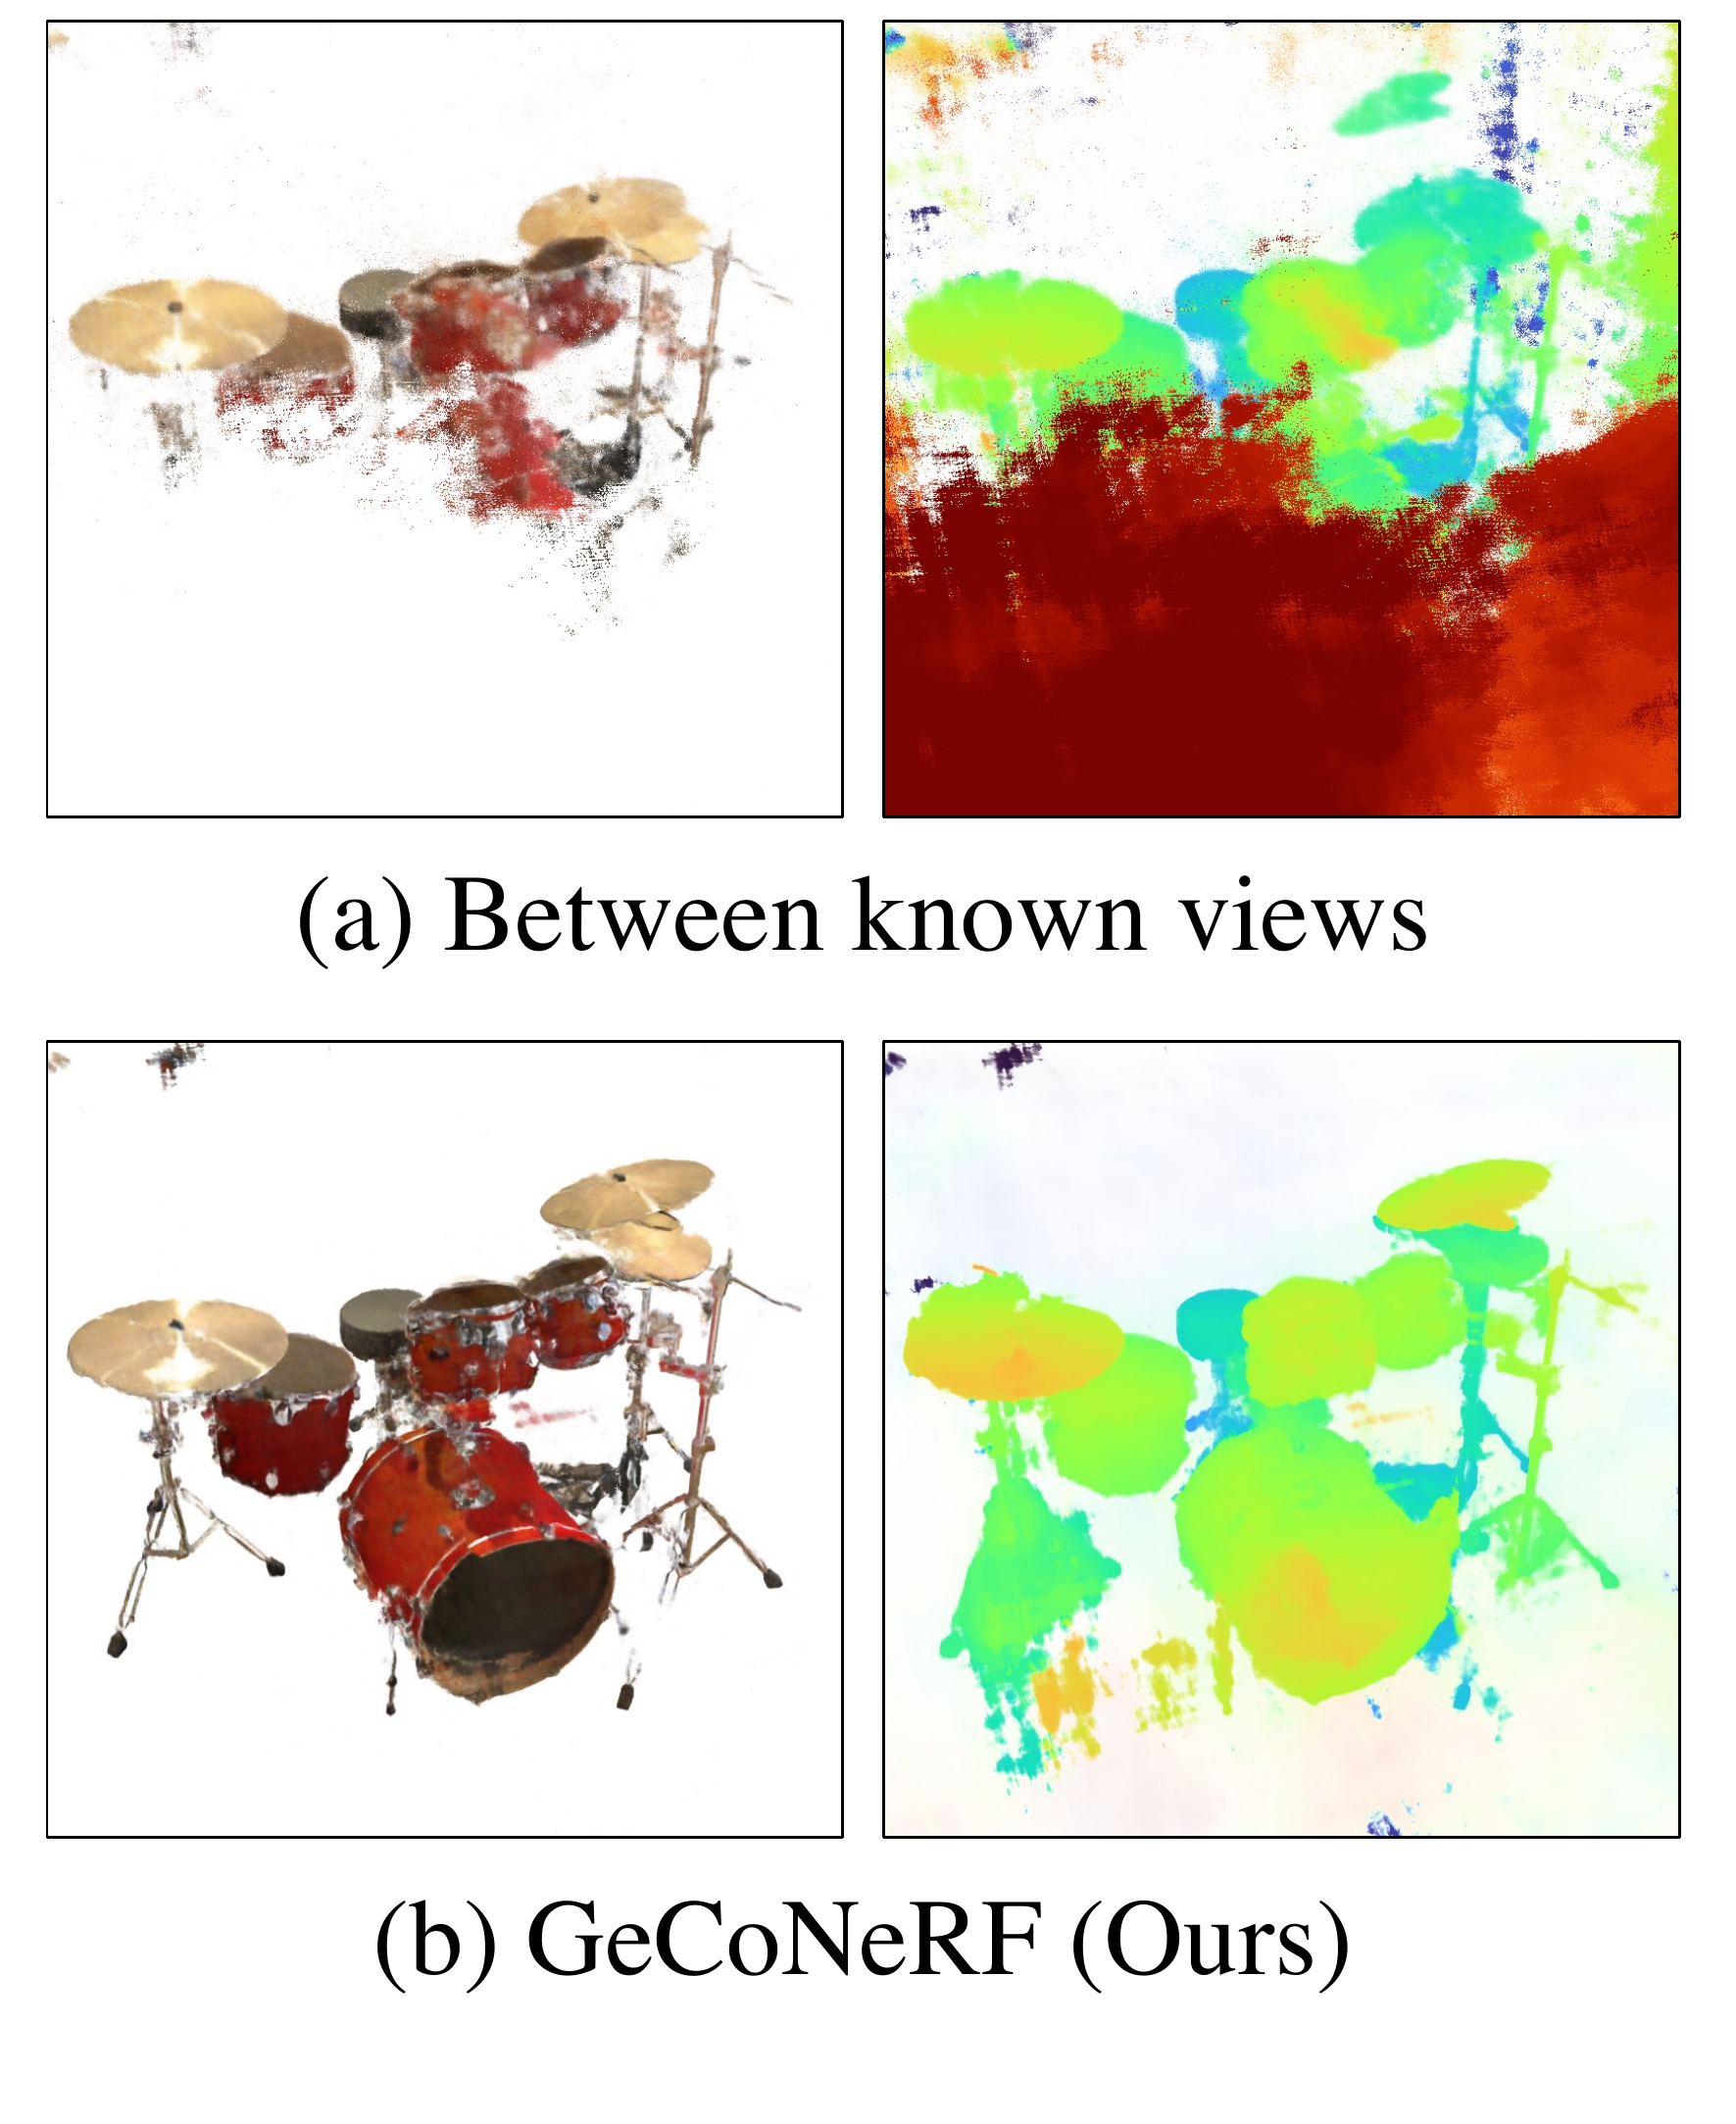}
  \end{center}
  \vspace{-24pt}
  \caption{
      \textbf{Consistency between known views vs. our method.}
  }
\label{qual:mvsfail}
\vspace{-20pt}
\end{wrapfigure}

It is standard practice in MVS~\cite{m3vsnet, khot2019learning} to model photometric consistency between ground truth view images, training the model to predict geometry in a self-supervised manner. Recent works in NeRF and neural SDF~\cite{mvsdf, neuralwarp, structnerf} adopt this method in standard "dense" view setting and show its effectiveness in refining geometry. However, this method has previous not been attempted in few-shot setting, and conduct an ablation study to see its effectiveness given our setting.

In order to compare GeCoNeRF with contemporary methods~\cite{neuralwarp, structnerf, geoNeuS} that model consistency between known views, we conduct an experiment to observe how such consistency modeling performs in few-shot NeRF setting. In our experiment, we replace our consistency modeling with above setting, warping source images to other known views for consistency between the warped image and ground truth (reference) image. 

Its result, shown in (a) of Figure~\ref{qual:mvsfail}, displays divergent behaviours such as heavy artifact generation, while our method (b) succeeds in recovering detailed geometry of the scene under the same setting. As discussed in Section~\ref{para:consistency}, we argue that large view differences and scarcity of reference images make it difficult for NeRF to refine geometry with consistency modeling between known views. Our work's novel contributions allow consistency modeling to be adopted to few-shot NeRF to facilitate stable training under such extreme conditions, distinguishing our work from above methods.

% \section{Robustness to input views}
\section{Robustness to Number of Input Views}
\label{viewnum}
To see the varying effects of our regularization loss regarding the number of input viewpoints, experimented on scenarios with 3, 6, 15 reference views on Blender dataset, and observed PSNR differences between our model and vanilla model in each setting. We selected 3, 6, 15 reference views, since RegNeRF and InfoNeRF both show saturating improvement against their baseline at ${15}$ reference views. The reason for our usage of 15 viewpoints, and not standard viewpoints (usually over 100), for abundant view setting is due to observations given in previous few-shot NeRF papers RegNeRF~\cite{Niemeyer2021Regnerf} and InfoNeRF~\cite{Kim2021Infonerf}: they observe that their vanilla baselines start to achieve better performance once enough input views are given, generally around 11-15, varying by the dataset. 
\vspace{-10pt}
% \begin{figure}
%     \centering
%     \includegraphics[width=\linewidth]{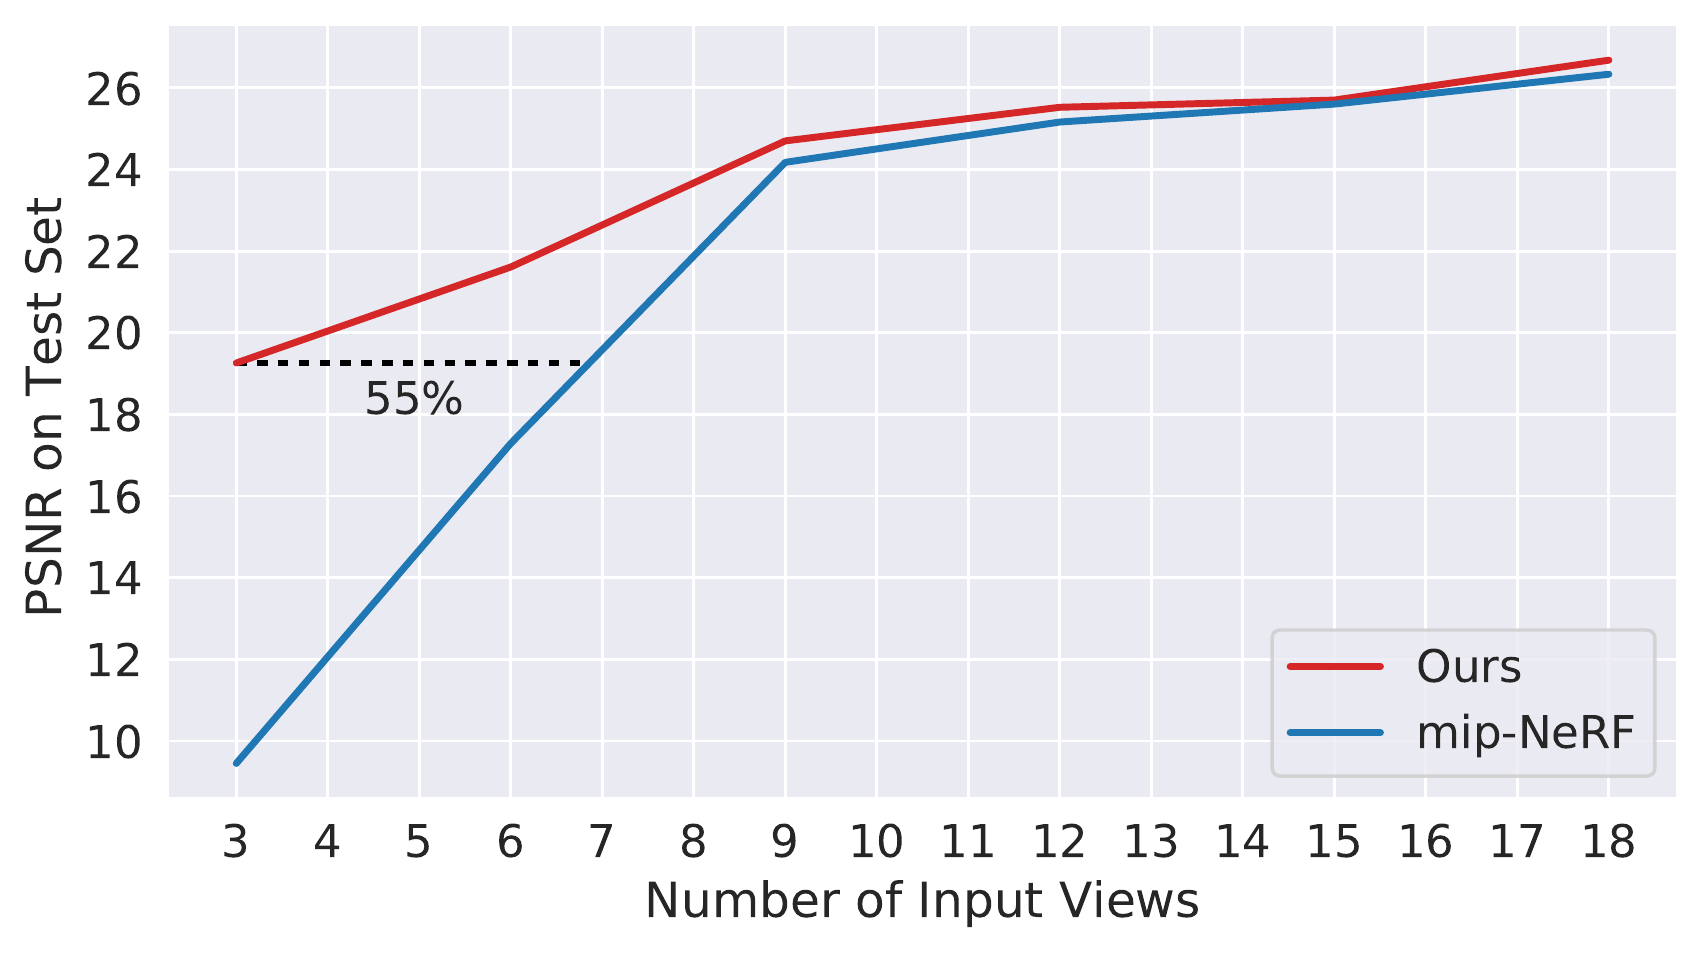}
%  \vspace{-.6cm}
%     \caption{
%         \textbf{Data Efficiency.}
%         In sparse settings, our method requires up to $55\%$ fewer images than mip-NeRF~\cite{barron2021mipnerf} to achieve a similar test set performance on the Blender dataset.
%         }
%     \label{fig:mipnerf_match}
%     \vspace{-10pt}
% \end{figure}

\begin{table}[!h]
\label{viewnum_table}
\centering

\caption{\textbf{Analysis with varying input view numbers.}} \vspace{5pt}
\scalebox{1}{
\setlength\tabcolsep{8pt} \hspace{-0.25cm}
\begin{tabular}{lcccc}
\toprule
Methods & 3 views  & 6 views & 15 views 
\\ 
\hline 
\hline
mip-NeRF~\cite{mildenhall2020nerf}  & 17.94 &	22.55  & \textbf{26.13}\\
\hdashline
GeCo-NeRF (Ours)&  \textbf{19.23}&	\textbf{22.89}	& 25.83 \\
\bottomrule
\end{tabular}
}
\vspace{-5pt}
\end{table}

As shown in Table 5, while our model displays better performance over our baseline model at few-shot settings, the difference between the two models becomes smaller as more input views are given. Finally, 15-view setting, our model is overtaken at by the baseline. This is consistent with results given in previous few-shot NeRF papers~\cite{Kim2021Infonerf, Niemeyer2021Regnerf} that commit to similar experiment. We speculate that NeRF reaches a point regarding inputs viewpoints where the regularization no longer benefits its optimization but rather constrains it from achieving higher performances.

\section{Limitations}
\label{limitations}
Our major limitations are as follows:

\textbf{(i)} Our method uses thresholding technique for occlusion handling and mask generation, and this makes our method sensitive to differences depending on different scenes and datasets. Even though we use singular threshold throughout different scenes, there are cases where small protrusions in the scene (such as lego blocks in Blender Lego scene) are masked out due to viewpoint-point based depth difference values that go just over the threshold values, and subjected less to novel viewpoint regularization. 

\textbf{(ii)} Our observed view consistency modeling depends on the assumption that there are large areas of surfaces that are covered by multiple viewpoints and thus able to be subjected to warping-based regularization. However, this validity of this assumption depends heavily on the nature of the scene and viewpoint selected, as there can be scenarios where a certain ground truth view shares no viewpoint with other ground truth views due to self-occlusion and large angular discrepancy between viewpoints. In such cases, all patches that are warped to the viewpoint would be masked out completely, resulting unnecessary computational cost for one third of the consistency modeling regularization steps.

\section{Broader Impact}
Our work enables few-shot optimization and rendering of NeRF, which allows neural radiance fields to be optimized with sparse images, which makes it more readily applicable to real-life applications, such 3D reconstruction and novel view synthesis. This in turn opens up new possibilities in multiple different ways, such as augmented reality, 3D scanning and easily manipulable visual effects.
